# Supplementary material for: Towards empirical force fields that match experimental observables
Source: arXiv:2004.01630 ancillary file (2020-05-29)
Supplement: Supplementary file 1 [file si.pdf]

# Supporting information for: Towards empirical force fields that match experimental observables

Thorben Fröhlking, Mattia Bernetti, Nicola Calonaci, and Giovanni Bussi

April 20, 2020

Table 1: Collection of force fields and their method for obtaining the respective parameter sets (reference to the initial paper is reported for each force field family as well as exemplary references to experiments or calculations, which were used). For comparison: Tetramer >120 atoms, Nucleotide 20 atoms + base, purine base 13 atoms + functional groups, pyrimidine base 10 atoms + functional groups. CCBD - Cambridge Crystal structure data bank, MC - Monte-Carlo-Simulations, HF- Hartree-Fock level of sprecision.

| | **AMBER**[1] | **CHARMM**[2] | **OPLS**[3] | **GROMOS**[4] |
|---|---|---|---|---|
| Bond | X-Ray,[5] Microwave-,[6] IR-spectroscopy[7] (hydrocarbons, NMA: 10-52 atoms) | CCDB survey,[8] Raman spectroscopy,[9,10] *Ab initio*[11] HF/3-21G, 4-21G (nucleobases: 12-16 atoms) | AMBER parameters | X-ray diffraction[12](aminoacids: 10-27 atoms) |
| Bend | X-Ray,[5] Microwave-,[6] IR-spectroscopy[7] (hydrocarbons, NMA: 10-52 atoms) | CCDB survey,[8] Raman spectroscopy,[9,10] *Ab initio*[11] HF/3-21G, 4-21G (nucleobases: 12-16 atoms) | AMBER parameters | X-ray diffraction[12](aminoacids: 10-27 atoms) |
| Torsion | *Ab initio* MP2/6-31G*, HF/6-31G*[13] and IR spectroscopy[14] (benzene, alanyl and glycyl dipeptides and NMA: 12-26 atoms) | CCDB survey,[8] Raman spectroscopy,[9,10] *Ab initio*[11] HF/3-21G, 4-21G (nucleobases: 12-16 atoms) | AMBER parameters | *Ab initio* HF 6-31G*[15] (backbone elements: 14 atoms) |
| LJ | MC (hydrocarbons: <14 atoms) + OPLS parameters | X-ray (adenyl-uridine , guanylyl-cytidine: 35, 37 atoms), gas-phase field ionization mass spectrometer,[16] *Ab initio* HF/3-21G, HF/6-31G* (nucleobases: 12-16 atoms) | MC of 36 organic liquids, Microwave spectroscopy,[17] density-,[18] vaporization calorimetry[19] and *Ab initio* HF/6-31G* | Distribution and dynamic vapor pressure experiments[20,21](aminoacids: 10-27 atoms) |
| Charges | RESP[22] (ESP: *Ab initio* HF/6-31G*) (hydrocarbons: 3-10 atoms) | OPLS charges + gas-phase field ionization mass spectrometry,[16] *Ab initio* HF/3-21G, HF/6-31G* (nucleobases: 12-16 atoms) | MC of 36 organic liquids, Microwave spectroscopy,[17] density-,[18] vaporization calorimetry[19] and *Ab initio* HF/6-31G* | Distribution and dynamic vapor pressure experiments[20,21](aminoacids: 10-27 atoms) |

## References


[1] Wendy D. Cornell, Piotr Cieplak, Christopher I. Bayly, Ian R. Gould, Kenneth M. Merz, David M. Ferguson, David C. Spellmeyer, Thomas Fox, James W. Caldwell, and Peter A. Kollman. A second generation force field for the simulation of proteins, nucleic acids, and organic molecules. *Journal of the American Chemical Society*, 117(19):5179–5197, 1995.

[2] Alexander D. MacKerell, Joanna Wiorkiewicz-Kuczera, and Martin Karplus. An all-atom empirical energy function for the simulation of nucleic acids. *Journal of the American Chemical Society*, 117(48):11946–11975, 1995.

[3] William L. Jorgensen and Julian Tirado-Rives. The opls [optimized potentials for liquid simulations] potential functions for proteins, energy minimizations for crystals of cyclic peptides and crambin. *Journal of the American Chemical Society*, 110(6):1657–1666, 1988. PMID: 27557051.

[4] Chris Oostenbrink, Alessandra Villa, Alan E. Mark, and Wilfred F. Van Gunsteren. A biomolecular force field based on the free enthalpy of hydration and solvation: The gromos force-field parameter sets 53a5 and 53a6. *Journal of Computational Chemistry*, 25(13):1656–1676, 2004.

[5] Scott J. Weiner, Peter A. Kollman, David A. Case, U. Chandra Singh, Caterina Ghio, Guliano Alagona, Salvatore Profeta, and Paul Weiner. A new force field for molecular mechanical simulation of nucleic acids and proteins. *Journal of the American Chemical Society*, 106(3):765–784, 1984.

[6] Marlin Harmony, Victor Laurie, Robert Kuczkowski, R Schwendeman, D Ramsay, Francis Lovas, Walter Lafferty, and Arthur Maki. Molecular structures of gas-phase polyatomic molecules determined by spectroscopic methods. *Journal of Physical and Chemical Reference Data*, 8:619–721, 07 1979.

[7] John Douglas, B. Rabinovitch, and F. Looney. Kinetics of the thermal cis-trans isomerization of dideuteroethylene. *The Journal of Chemical Physics*, 23:315–323, 02 1955.

[8] Robin Taylor and Olga Kennard. The molecular structures of nucleosides and nucleotides: Part 1. the influence of protonation on the geometries of nucleic acid constituents. *Journal of Molecular Structure*, 78(1):1 – 28, 1982.

[9] A.J. Barnes, M.A. Stuckey, and L. Le Gall. Nucleic acid bases studied by matrix isolation vibrational spectroscopy: Uracil and deuterated uracils. *Spectrochimica Acta Part A: Molecular Spectroscopy*, 40(5):419 – 431, 1984.

[10] L. Harsányi, P. Császár, A. Császár, and J. E. Boggs. Interpretation of the vibrational spectra of matrix-isolated uracil from scaled ab initio quantum mechanical force fields. *International Journal of Quantum Chemistry*, 29(4):799–815, 1986.

[11] Misako Aida. An ab initio molecular orbital study on the sequence-dependency of dna conformation: An evaluation of intra- and inter-strand stacking interaction energy. *Journal of Theoretical Biology*, 130(3):327 – 335, 1988.

[12] W. F. Van Gunsteren and M. Karplus. Protein dynamics in solution and in a crystalline environment: a molecular dynamics study. *Biochemistry*, 21(10):2259–2274, 1982. PMID: 6178423.

[13] Ian R. Gould and Peter A. Kollman. Ab initio scf and mp2 calculations on four low-energy conformers of n-acetyl-n'-methylalaninamide. *The Journal of Physical Chemistry*, 96(23):9255–9258, 1992.

[14] Madeleine Rey-Lafon, M. T. Forel, and C. Garrigou-Lagrange. Discussion des modes normaux des groupements amides cis et trans à partir des champs de force du $\sigma$-valérolactame et du n methylacetamide. 1973.

[15] Thereza A. Soares, Philippe H. Hünenberger, Mika A. Kastenholz, Vincent Kräutler, Thomas Lenz, Roberto D. Lins, Chris Oostenbrink, and Wilfred F. van Gunsteren. An improved nucleic acid parameter set for the gromos force field. *Journal of Computational Chemistry*, 26(7):725–737, 2005.

[16] I. K. Yanson, A. B. Teplitsky, and L. F. Sukhodub. Experimental studies of molecular interactions between nitrogen bases of nucleic acids. *Biopolymers*, 18(5):1149–1170, 1979.

[17] J. R. Durig and D. A. C. Compton. Analysis of torsional spectra of molecules with two internal c3v rotors. 15. low-frequency vibrational spectra, methyl torsional potential functions, and molecular structure of ethylmethylamine. *The Journal of Physical Chemistry*, 83(22):2873–2879, 1979.

[18] Lars Bøje and Aase Hvidt. Densities of aqueous mixtures of non-electrolytes. *The Journal of Chemical Thermodynamics*, 3(5):663 – 673, 1971.

[19] G. Somsen and J. Coops. Enthalpies of solvation of alkali halides in formamide. i: The enthalpies of solution of alkali halides in formamide. *Recueil des Travaux Chimiques des Pays-Bas*, 84(8):985–1002, 1965.

[20] Anna Radzicka and Richard Wolfenden. Comparing the polarities of the amino acids: side-chain distribution coefficients between the vapor phase, cyclohexane, 1-octanol, and neutral aqueous solution. *Biochemistry*, 27(5):1664–1670, 1988.

[21] R. Wolfenden, L. Andersson, P. M. Cullis, and C. C. B. Southgate. Affinities of amino acid side chains for solvent water. *Biochemistry*, 20(4):849–855, 1981. PMID: 7213619.

[22] James W. Caldwell and Peter A. Kollman. Structure and properties of neat liquids using nonadditive molecular dynamics: Water, methanol, and n-methylacetamide. *The Journal of Physical Chemistry*, 99(16):6208–6219, 1995.
